# Supplementary material for: Uncertainty Quantification in Federated Granger Causality Learning
Source: arXiv:2602.13004 source file (2026-10-08)
Supplement: Supplementary file 1 [file AdditionalTheory.tex]

% \subsection{Lemma \ref{lemma:client_grad_cov_means}}
% \begin{lemma}\label{lemma:client_grad_cov_means}
% At any time $t$ and, for each client $m$, define
% \[
% g_m \;=\; \nabla_{\theta_m} L_s
% \;=\; X_m\,(y_m^{t-1})^{\top}, 
% \qquad
% X_m := A_{mm}^{\top}\!\Big(A_{mm}\,\Delta h_m - \sum_{r\neq m}\hat A_{mr}(\hat h^{t-1}_r)_c\Big).
% \]
% Under Assumptions \textbf{(A1)}-\textbf{(A4)}, we have for any $m \neq n$,
% \[
% \operatorname{Cov}\!\big(\mathrm{vec}(g_m),\,\mathrm{vec}(g_n)\big) \;=\; 0.
% \]
% \end{lemma}
% \begin{proof}
% By Assumption \textbf{(A2)}, the block-row server parameters for clients $m$ and $n$ are mutually independent, hence $X_m \perp X_n$.  
% By Assumptions \textbf{(A1)}, \textbf{(A4)}, and \textbf{(A5)}, the local data satisfy
% \[
% \mu_{y_m} = \mathbb{E}[y_m^{t-1}], 
% \qquad 
% \Sigma_{y_m} = \operatorname{Cov}(y_m^{t-1}, y_m^{t-1}),
% \]
% with $\operatorname{Cov}(y_m^{t-1},y_n^{t-1})=0$ for $m\neq n$.  
% Since $y_m^{t-1}$ is also independent of $\{A_{pq}^t\}$ by Assumption \textbf{(A3)}, we may write
% \[
% \mathrm{vec}(g_m) = (I \otimes X_m)\,y_m^{t-1}.
% \]
% Thus, for $m\neq n$,
% \[
% \operatorname{Cov}\!\big(\mathrm{vec}(g_m),\mathrm{vec}(g_n)\big)
% = \mathbb{E}\!\big[(I\otimes X_m)\,y_m^{t-1}(y_n^{t-1})^{\top}(I\otimes X_n)^{\top}\big]
% - \mathbb{E}[\mathrm{vec}(g_m)]\,\mathbb{E}[\mathrm{vec}(g_n)]^{\top}.
% \]
% Independence allows factorization, and Assumption \textbf{(A4)}--\textbf{(A5)} implies
% $\mathbb{E}[y_m^{t-1}(y_n^{t-1})^{\top}]=\mu_{y_m}\mu_{y_n}^{\top}$, 
% which cancels with the product of means. Hence
% \[
% \operatorname{Cov}\!\big(\mathrm{vec}(g_m),\mathrm{vec}(g_n)\big) = 0,
% \quad m \neq n.
% \]
% \end{proof}

% \subsection{Proposition~\ref{prop:theta_indep}}
% \begin{proposition}\label{prop:theta_indep}
% Consider the client update rule
% \[
% \theta_m^{t+1} \;=\; \theta_m^t - \eta_1 g_{m,a}^t - \eta_2 g_{m,s}^t,
% \]
% where $g_{m,a}^t = \nabla_{\theta_m} L_m$ (local) and $g_{m,s}^t = \nabla_{\theta_m} L_s$ (global).  
% Suppose Assumptions \textbf{(A1)}--\textbf{(A5)} hold. Then, for any two distinct clients $m \neq n$,
% \[
% \lim_{t \to \infty}\operatorname{Cov}(\theta_m^t, \theta_n^t) \;=\; 0.
% \]
% \end{proposition}

% \begin{proof}
% Expanding the covariance for $m\neq n$ gives
% \begin{align*}
% \operatorname{Cov}(\theta_m^{t+1}, \theta_n^{t+1})
% = \operatorname{Cov}(\theta_m^t,\theta_n^t)
% + \eta_2^2 \operatorname{Cov}(g_{m,s}^t,g_{n,s}^t) + \text{vanishing local terms}
% \end{align*}
% where the omitted terms involve cross-products between local and global gradients.  

% By Lemma~\ref{lemma:client_grad_cov_means}, $\operatorname{Cov}(g_{m,s}^t,g_{n,s}^t)=0$ for $m\neq n$.  
% By \textbf{(A2)} and \textbf{(A3)}, $\theta_m^t \perp\!\!\!\perp \theta_n^t$ at initialization.  
% By \textbf{(A4)}--\textbf{(A5)}, client data are uncorrelated across $m,n$, and all noise is additive.  
% Hence all cross-terms vanish, and we obtain the recursion
% \[
% \operatorname{Cov}(\theta_m^{t+1},\theta_n^{t+1})
% = \operatorname{Cov}(\theta_m^t,\theta_n^t).
% \]
% Since the initial covariance is zero, induction gives
% \(\operatorname{Cov}(\theta_m^t,\theta_n^t)=0\) for all $t$, and thus
% \[
% \lim_{t\to\infty}\operatorname{Cov}(\theta_m^t,\theta_n^t)=0.
% \]
% \end{proof}

% \subsection{Proposition~\ref{prop:data-var-R}}
% As a direct consequence of Assumption \textbf{(A5)} we have the following proposition: 
% \begin{proposition}[\textbf{Data Uncertainty with Zero Process Noise}]
% \label{prop:data-var-R}
% Consider the discrete LTI system
% \begin{equation*}
%     x^{t+1}=A\,x^t + w^t, 
% \hspace{0.2cm}
% y^t=C\,x^t+v^t,
% \hspace{0.2cm} 
% w^t \sim\mathcal N(0, Q), \hspace{0.1cm} \text{and} \hspace{0.1cm} v^t\sim\mathcal N(0,R)
% \end{equation*}
% and assume the state matrix is asymptotically stable,
% \(\rho(A)<1\).
% In the absence of process noise i.e., $Q = 0$, then the data variance converges to its noise covariance.  
% \(
% \lim_{t\to\infty}\operatorname{Var}(y^t)=R.
% \)
% \end{proposition}
% \begin{proof}
% With \( Q = 0 \), the state update becomes deterministic:
% \[
% x^{t+1} = A x^t.
% \]
% Thus, assuming some initial condition \( x^0 \), the state at time \( t \) is given by, 
% \[
% x^t = A^t x^0.
% \]
% Therefore, the data $y^t$ is given by, 
% \[
% y^t = C x^t + v^t = C A^t x^0 + v^t.
% \]

% To compute the variance of \( y^t \), we consider the following equation, 
% \[
% \operatorname{Var}(y^t) = \operatorname{Var}(C A^t x^0 + v^t).
% \]

% Since \( v^t \sim \mathcal{N}(0, R) \) is independent of \( x^0 \), and \( C A^t x^0 \) is deterministic, we write $\operatorname{Var}(y^t)$ as, 
% \[
% \operatorname{Var}(y^t) = \operatorname{Var}(C A^t x^0) + \operatorname{Var}(v^t).
% \]

% Now, since \( C A^t x^0 \) is deterministic, its variance is given by, 
% \[
% \operatorname{Var}(C A^t x^0) = C A^t \operatorname{Var}(x^0) (A^t)^\top C^\top.
% \]

% Given that \( \rho(A) < 1 \), we have \( A^t \to 0 \) as \( t \to \infty \) we have, 
% \[
% C A^t \operatorname{Var}(x^0) (A^t)^\top C^\top \to 0.
% \]

% Using the above result, and the fact that $\operatorname{Var}(v^t) = R$ we can write $\operatorname{Var}(y^t)$ as, 
% \[
% \lim_{t \to \infty} \operatorname{Var}(y^t) = \lim_{t \to \infty} \left[ C A^t \operatorname{Var}(x^0) (A^t)^\top C^\top + R \right] = R.
% \]
% \end{proof}
