# Supplementary material for: Uncertainty Quantification in Federated Granger Causality Learning
Source: arXiv:2602.13004 source file (2026-10-08)
Supplement: Supplementary file 2 [file Images.tex]

% \begin{figure}[H]
%   \centering
%   % Row 1
%   \begin{subfigure}[b]{0.33\columnwidth}
%     \centering
%     \includegraphics[width=\textwidth]{Figures/SyntheticDataset/Epistemic/sigma_Amn/Trace_Cov_A_mn_21.pdf}
%     \caption{} \label{1a}
%   \end{subfigure}%
%   \begin{subfigure}[b]{0.33\columnwidth}
%     \centering
%     \includegraphics[width=\textwidth]{Figures/SyntheticDataset/Epistemic/sigma_Amn/Trace_Cov_theta_2.pdf}
%     \caption{} \label{1b}
%   \end{subfigure}%
%   \begin{subfigure}[b]{0.33\columnwidth}
%     \centering
%     \includegraphics[width=\textwidth]{Figures/SyntheticDataset/Epistemic/sigma_Amn/L2_Norm_Avg_Error_21.pdf}
%     \caption{} \label{1c}
%   \end{subfigure}
%   \begin{subfigure}[b]{0.33\columnwidth}
%     \centering
%     \includegraphics[width=\textwidth]{Figures/SyntheticDataset/Epistemic/sigma_theta/Trace_Cov_A_mn_21.pdf}
%     \caption{} \label{1a}
%   \end{subfigure}%
%   \begin{subfigure}[b]{0.33\columnwidth}
%     \centering
%     \includegraphics[width=\textwidth]{Figures/SyntheticDataset/Epistemic/sigma_theta/Trace_Cov_theta_2.pdf}
%     \caption{} \label{1b}
%   \end{subfigure}%
%   \begin{subfigure}[b]{0.33\columnwidth}
%     \centering
%     \includegraphics[width=\textwidth]{Figures/SyntheticDataset/Epistemic/sigma_theta/L2_Norm_Avg_Error_21.pdf}
%     \caption{} \label{1c}
%   \end{subfigure}
%   \caption{%
%   Uncertainty prop. highlighting
%     (a) $\mathrm{Tr}(\Sigma_{\hat{A}_{21}^t})$, 
%     (b) $\mathrm{Tr}(\Sigma_{\theta_2}^t)$, 
%     (c) $\|\mu_{\hat{A}_{21}^t}-A_{21}\|_2$ vs iter. $t$ for different levels of $\Sigma_{\hat{A}_{mn}^0}$ (top row), and $\Sigma_{\theta_m}^0$ (bottom row)
%   }
%   \label{fig:epistemic_sigma_theta}
% \end{figure}


% \begin{figure}[H]
%   \centering
%   \begin{subfigure}[b]{0.33\columnwidth}
%     \centering
%     \includegraphics[width=\textwidth]{Appendix/Figures/cross_covariance/aleatoric/Trace_CrossCov_A_mn_Xvfl_21.pdf}
%     \caption{} \label{1a}
%   \end{subfigure}%
%   \begin{subfigure}[b]{0.33\columnwidth}
%     \centering
%     \includegraphics[width=\textwidth]{Appendix/Figures/cross_covariance/aleatoric/Trace_CrossCov_theta_Xvfl_2.pdf}
%     \caption{} \label{1b}
%   \end{subfigure}%
%   \begin{subfigure}[b]{0.33\columnwidth}
%     \centering
%     \includegraphics[width=\textwidth]{Appendix/Figures/cross_covariance/aleatoric/Trace_CrossCov_A_mn_theta_21.pdf}
%     \caption{} \label{1c}
%   \end{subfigure}

%   \caption{%
%     Uncertainty propagation in the cross-covariance terms during FedGC learning for different regimes of $\Sigma_{y_m}^t$
%     (a) $\Gamma_{21}^t$ vs iterations, 
%     (b) $\Lambda_2^t$ vs iterations, 
%     (c) $\Psi_{21}^t$ vs iterations.%
%   in the synthetic dataset}
%   \label{fig:aleatoric_cross_cov_sigma_y}
% \end{figure}

% \begin{figure}[H]
%   \centering
%   \begin{subfigure}[b]{0.33\columnwidth}
%     \centering
%     \includegraphics[width=\textwidth]{Appendix/Figures/cross_covariance/epistemic/sigma_Amn/Trace_CrossCov_A_mn_Xvfl_21.pdf}
%     \caption{} \label{1a}
%   \end{subfigure}%
%   \begin{subfigure}[b]{0.33\columnwidth}
%     \centering
%     \includegraphics[width=\textwidth]{Appendix/Figures/cross_covariance/epistemic/sigma_Amn/Trace_CrossCov_theta_Xvfl_2.pdf}
%     \caption{} \label{1b}
%   \end{subfigure}%
%   \begin{subfigure}[b]{0.33\columnwidth}
%     \centering
%     \includegraphics[width=\textwidth]{Appendix/Figures/cross_covariance/epistemic/sigma_Amn/Trace_CrossCov_A_mn_theta_21.pdf}
%     \caption{} \label{1c}
%   \end{subfigure}

%   \caption{%
%     Uncertainty propagation in the cross-covariance terms during FedGC learning for different regimes of $\Sigma_{\hat{A}_{mn}}^0$
%     (a) $\Gamma_{21}^t$ vs iterations, 
%     (b) $\Lambda_2^t$ vs iterations, 
%     (c) $\Psi_{21}^t$ vs iterations.%
%   in the synthetic dataset}
%   \label{fig:epistemic_cross_cov_Sigma_Amn}
% \end{figure}

% \begin{figure}[H]
%   \centering
%   \begin{subfigure}[b]{0.33\columnwidth}
%     \centering
%     \includegraphics[width=\textwidth]{Appendix/Figures/cross_covariance/epistemic/sigma_theta/Trace_CrossCov_A_mn_Xvfl_21.pdf}
%     \caption{} \label{1a}
%   \end{subfigure}%
%   \begin{subfigure}[b]{0.33\columnwidth}
%     \centering
%     \includegraphics[width=\textwidth]{Appendix/Figures/cross_covariance/epistemic/sigma_theta/Trace_CrossCov_theta_Xvfl_2.pdf}
%     \caption{} \label{1b}
%   \end{subfigure}%
%   \begin{subfigure}[b]{0.33\columnwidth}
%     \centering
%     \includegraphics[width=\textwidth]{Appendix/Figures/cross_covariance/epistemic/sigma_theta/Trace_CrossCov_A_mn_theta_21.pdf}
%     \caption{} \label{1c}
%   \end{subfigure}

%   \caption{%
%     Uncertainty propagation in the cross-covariance terms during FedGC learning for different regimes of $\Sigma_{\theta_m^t}$
%     (a) $\Gamma_{21}^t$ vs iterations, 
%     (b) $\Lambda_2^t$ vs iterations, 
%     (c) $\Psi_{21}^t$ vs iterations.%
%   in the synthetic dataset}
%   \label{fig:epistemic_cross_cov_Sigma_theta}
% \end{figure}

% \begin{figure}[H]
%   \centering
%   \begin{subfigure}[b]{0.4\columnwidth}
%     \centering
%     \includegraphics[width=\textwidth]{Appendix/Figures/communicated_quantities/aleatoric/Trace_Cov_X_vfl_pred_2.pdf}
%     \caption{} \label{1a}
%   \end{subfigure}%
%   \begin{subfigure}[b]{0.4\columnwidth}
%     \centering
%     \includegraphics[width=\textwidth]{Appendix/Figures/communicated_quantities/aleatoric/Trace_Cov_Ls_gradx_iter_2.pdf}
%     \caption{} \label{1b}
%   \end{subfigure}%
%   \caption{%
%     Uncertainty propagation in the communicated terms during FedGC learning for different regimes of $\Sigma_{y_m}^t$
%     (a) $\operatorname{Var}\bigl(g_{m, s}^{\,t}\bigr)$ vs iterations, 
%     (b) $\Sigma_{h_m}^t$ vs iterations, 
%   in the synthetic dataset}
%   \label{fig:aleatoric_comm_sigma_y}
% \end{figure}

% \begin{figure}[H]
%   \centering
%   \begin{subfigure}[b]{0.4\columnwidth}
%     \centering
%     \includegraphics[width=\textwidth]{Appendix/Figures/communicated_quantities/epistemic/sigma_Amn/Trace_Cov_X_vfl_pred_2.pdf}
%     \caption{} \label{1a}
%   \end{subfigure}%
%   \begin{subfigure}[b]{0.4\columnwidth}
%     \centering
%     \includegraphics[width=\textwidth]{Appendix/Figures/communicated_quantities/epistemic/sigma_Amn/Trace_Cov_Ls_gradx_iter_2.pdf}
%     \caption{} \label{1b}
%   \end{subfigure}%
%   \caption{%
%     Uncertainty propagation in the communicated terms during FedGC learning for different regimes of $\Sigma_{\hat{A}_{mn}^0}$
%     (a) $\operatorname{Var}\bigl(g_{m, s}^{\,t}\bigr)$ vs iterations, 
%     (b) $\Sigma_{h_m}^t$ vs iterations, 
%   in the synthetic dataset}
%   \label{fig:aleatoric_comm_sigma_Amn}
% \end{figure}

% \begin{figure}[H]
%   \centering
%   \begin{subfigure}[b]{0.4\columnwidth}
%     \centering
%     \includegraphics[width=\textwidth]{Appendix/Figures/communicated_quantities/epistemic/sigma_theta/Trace_Cov_X_vfl_pred_2.pdf}
%     \caption{} \label{1a}
%   \end{subfigure}%
%   \begin{subfigure}[b]{0.4\columnwidth}
%     \centering
%     \includegraphics[width=\textwidth]{Appendix/Figures/communicated_quantities/epistemic/sigma_theta/Trace_Cov_Ls_gradx_iter_2.pdf}
%     \caption{} \label{1b}
%   \end{subfigure}%
%   \caption{%
%     Uncertainty propagation in the communicated terms during FedGC learning for different regimes of $\Sigma_{\theta_m^t}$
%     (a) $\operatorname{Var}\bigl(g_{m, s}^{\,t}\bigr)$ vs iterations, 
%     (b) $\Sigma_{h_{m}}^t$ vs iterations, 
%   in the synthetic dataset}
%   \label{fig:aleatoric_comm_sigma_theta}
% \end{figure}

% \begin{figure}[H]
%   \centering
%   \includegraphics[width=0.4\columnwidth]{Appendix/Figures/RealworldDataset/hai/nonlinear/aleatoric/Server_Loss.pdf}
%   \caption{Nonlinear Exper. on HAI: Training loss of the server model for different $\Sigma_{y_m}^t$}
%   \label{fig:server_loss_hai_nonlinear}
% \end{figure}

% \begin{figure}[H]
%   \centering
%   % Row 1
%   \begin{subfigure}[b]{0.33\columnwidth}
%     \centering
%     \includegraphics[width=\textwidth]{Appendix/Figures/RealworldDataset/hai/aleatoric/L2_Norm_Avg_Error_12.pdf}
%     \caption{$\|\mu_{\hat{A}_{12}^t}-A_{12}\|_2$}\label{fig:L2Error12}
%   \end{subfigure}%
%   \begin{subfigure}[b]{0.33\columnwidth}
%     \centering
%     \includegraphics[width=\textwidth]{Appendix/Figures/RealworldDataset/hai/aleatoric/L2_Norm_Avg_Error_13.pdf}
%     \caption{$\|\mu_{\hat{A}_{13}^t}-A_{13}\|_2$}\label{fig:L2Error13}
%   \end{subfigure}%
%   \begin{subfigure}[b]{0.33\columnwidth}
%     \centering
%     \includegraphics[width=\textwidth]{Appendix/Figures/RealworldDataset/hai/aleatoric/L2_Norm_Avg_Error_21.pdf}
%     \caption{$\|\mu_{\hat{A}_{21}^t}-A_{21}\|_2$}\label{fig:L2Error21}
%   \end{subfigure}

%   \vskip\baselineskip

%   % Row 2
%   \begin{subfigure}[b]{0.33\columnwidth}
%     \centering
%     \includegraphics[width=\textwidth]{Appendix/Figures/RealworldDataset/hai/aleatoric/L2_Norm_Avg_Error_23.pdf}
%     \caption{$\|\mu_{\hat{A}_{23}^t}-A_{23}\|_2$}\label{fig:L2Error23}
%   \end{subfigure}%
%   \begin{subfigure}[b]{0.33\columnwidth}
%     \centering
%     \includegraphics[width=\textwidth]{Appendix/Figures/RealworldDataset/hai/aleatoric/L2_Norm_Avg_Error_31.pdf}
%     \caption{$\|\mu_{\hat{A}_{31}^t}-A_{31}\|_2$}\label{fig:L2Error31}
%   \end{subfigure}%
%   \begin{subfigure}[b]{0.33\columnwidth}
%     \centering
%     \includegraphics[width=\textwidth]{Appendix/Figures/RealworldDataset/hai/aleatoric/L2_Norm_Avg_Error_32.pdf}
%     \caption{$\|\mu_{\hat{A}_{32}^t}-A_{32}\|_2$}\label{fig:L2Error32}
%   \end{subfigure}

%   \caption{Average $L_2$ norm error of each off-diagonal block of the matrix $A$ for different regimes of $\Sigma_{y_m}^t$ for HAI dataset}
%   \label{fig:L2_error_offdiag_A_realworld}
% \end{figure}

% \begin{figure}[H]
%   \centering
%   % Row 1
%   \begin{subfigure}[b]{0.33\columnwidth}
%     \centering
%     \includegraphics[width=\textwidth]{Appendix/Figures/RealworldDataset/hai/epistemic/sigma_Amn/L2_Norm_Avg_Error_12.pdf}
%     \caption{$\|\mu_{\hat{A}_{12}^t}-A_{12}\|_2$}\label{fig:L2Error12}
%   \end{subfigure}%
%   \begin{subfigure}[b]{0.33\columnwidth}
%     \centering
%     \includegraphics[width=\textwidth]{Appendix/Figures/RealworldDataset/hai/epistemic/sigma_Amn/L2_Norm_Avg_Error_13.pdf}
%     \caption{$\|\mu_{\hat{A}_{13}^t}-A_{13}\|_2$}\label{fig:L2Error13}
%   \end{subfigure}%
%   \begin{subfigure}[b]{0.33\columnwidth}
%     \centering
%     \includegraphics[width=\textwidth]{Appendix/Figures/RealworldDataset/hai/epistemic/sigma_Amn/L2_Norm_Avg_Error_21.pdf}
%     \caption{$\|\mu_{\hat{A}_{21}^t}-A_{21}\|_2$}\label{fig:L2Error21}
%   \end{subfigure}

%   \vskip\baselineskip

%   % Row 2
%   \begin{subfigure}[b]{0.33\columnwidth}
%     \centering
%     \includegraphics[width=\textwidth]{Appendix/Figures/RealworldDataset/hai/epistemic/sigma_Amn/L2_Norm_Avg_Error_23.pdf}
%     \caption{$\|\mu_{\hat{A}_{23}^t}-A_{23}\|_2$}\label{fig:L2Error23}
%   \end{subfigure}%
%   \begin{subfigure}[b]{0.33\columnwidth}
%     \centering
%     \includegraphics[width=\textwidth]{Appendix/Figures/RealworldDataset/hai/epistemic/sigma_Amn/L2_Norm_Avg_Error_31.pdf}
%     \caption{$\|\mu_{\hat{A}_{31}^t}-A_{31}\|_2$}\label{fig:L2Error31}
%   \end{subfigure}%
%   \begin{subfigure}[b]{0.33\columnwidth}
%     \centering
%     \includegraphics[width=\textwidth]{Appendix/Figures/RealworldDataset/hai/epistemic/sigma_Amn/L2_Norm_Avg_Error_32.pdf}
%     \caption{$\|\mu_{\hat{A}_{32}^t}-A_{32}\|_2$}\label{fig:L2Error32}
%   \end{subfigure}

%   \caption{Average $L_2$ norm error of each off-diagonal block of the matrix $A$ for different regimes of $\Sigma_{\hat{A}_{mn}}^0$ for HAI dataset}
%   \label{fig:L2_error_offdiag_A_hai}
% \end{figure}

% \begin{figure}[H]
%   \centering
%   % Row 1
%   \begin{subfigure}[b]{0.33\columnwidth}
%     \centering
%     \includegraphics[width=\textwidth]{Appendix/Figures/RealworldDataset/hai/nonlinear/aleatoric/Trace_Cov_J_mn_12.pdf}
%     \caption{$\mathrm{Tr}\bigl(\Sigma_{\hat{J}_{12}^t}\bigr)$}\label{fig:traceJ12}
%   \end{subfigure}%
%   \begin{subfigure}[b]{0.33\columnwidth}
%     \centering
%     \includegraphics[width=\textwidth]{Appendix/Figures/RealworldDataset/hai/nonlinear/aleatoric/Trace_Cov_J_mn_13.pdf}
%     \caption{$\mathrm{Tr}\bigl(\Sigma_{\hat{J}_{13}^t}\bigr)$}\label{fig:traceJ13}
%   \end{subfigure}%
%   \begin{subfigure}[b]{0.33\columnwidth}
%     \centering
%     \includegraphics[width=\textwidth]{Appendix/Figures/RealworldDataset/hai/nonlinear/aleatoric/Trace_Cov_J_mn_21.pdf}
%     \caption{$\mathrm{Tr}\bigl(\Sigma_{\hat{J}_{21}^t}\bigr)$}\label{fig:traceJ21}
%   \end{subfigure}

%   \vskip\baselineskip

%   % Row 2
%   \begin{subfigure}[b]{0.33\columnwidth}
%     \centering
%     \includegraphics[width=\textwidth]{Appendix/Figures/RealworldDataset/hai/nonlinear/aleatoric/Trace_Cov_J_mn_23.pdf}
%     \caption{$\mathrm{Tr}\bigl(\Sigma_{\hat{J}_{23}^t}\bigr)$}\label{fig:traceJ23}
%   \end{subfigure}%
%   \begin{subfigure}[b]{0.33\columnwidth}
%     \centering
%     \includegraphics[width=\textwidth]{Appendix/Figures/RealworldDataset/hai/nonlinear/aleatoric/Trace_Cov_J_mn_31.pdf}
%     \caption{$\mathrm{Tr}\bigl(\Sigma_{\hat{J}_{31}^t}\bigr)$}\label{fig:traceJ31}
%   \end{subfigure}%
%   \begin{subfigure}[b]{0.33\columnwidth}
%     \centering
%     \includegraphics[width=\textwidth]{Appendix/Figures/RealworldDataset/hai/nonlinear/aleatoric/Trace_Cov_J_mn_32.pdf}
%     \caption{$\mathrm{Tr}\bigl(\Sigma_{\hat{J}_{32}^t}\bigr)$}\label{fig:traceJ32}
%   \end{subfigure}

%   \caption{Nonlinear Exper. on HAI: Trace of the covariance for the off-diagonal blocks of the Jacobian matrix $J$  for different $\Sigma_{y_m}^t$}
%   \label{fig:trace_cov_offdiag_J_hai}
% \end{figure}

% \begin{figure}[H]
%   \centering
%   % Row 1
%   \begin{subfigure}[b]{0.33\columnwidth}
%     \centering
%     \includegraphics[width=\textwidth]{Appendix/Figures/RealworldDataset/hai/nonlinear/epistemic/Trace_Cov_J_mn_12.pdf}
%     \caption{$\mathrm{Tr}\bigl(\Sigma_{\hat{J}_{12}^t}\bigr)$}\label{fig:traceJ12}
%   \end{subfigure}%
%   \begin{subfigure}[b]{0.33\columnwidth}
%     \centering
%     \includegraphics[width=\textwidth]{Appendix/Figures/RealworldDataset/hai/nonlinear/epistemic/Trace_Cov_J_mn_13.pdf}
%     \caption{$\mathrm{Tr}\bigl(\Sigma_{\hat{J}_{13}^t}\bigr)$}\label{fig:traceJ13}
%   \end{subfigure}%
%   \begin{subfigure}[b]{0.33\columnwidth}
%     \centering
%     \includegraphics[width=\textwidth]{Appendix/Figures/RealworldDataset/hai/nonlinear/epistemic/Trace_Cov_J_mn_21.pdf}
%     \caption{$\mathrm{Tr}\bigl(\Sigma_{\hat{J}_{21}^t}\bigr)$}\label{fig:traceJ21}
%   \end{subfigure}

%   \vskip\baselineskip

%   % Row 2
%   \begin{subfigure}[b]{0.33\columnwidth}
%     \centering
%     \includegraphics[width=\textwidth]{Appendix/Figures/RealworldDataset/hai/nonlinear/epistemic/Trace_Cov_J_mn_23.pdf}
%     \caption{$\mathrm{Tr}\bigl(\Sigma_{\hat{J}_{23}^t}\bigr)$}\label{fig:traceJ23}
%   \end{subfigure}%
%   \begin{subfigure}[b]{0.33\columnwidth}
%     \centering
%     \includegraphics[width=\textwidth]{Appendix/Figures/RealworldDataset/hai/nonlinear/epistemic/Trace_Cov_J_mn_31.pdf}
%     \caption{$\mathrm{Tr}\bigl(\Sigma_{\hat{J}_{31}^t}\bigr)$}\label{fig:traceJ31}
%   \end{subfigure}%
%   \begin{subfigure}[b]{0.33\columnwidth}
%     \centering
%     \includegraphics[width=\textwidth]{Appendix/Figures/RealworldDataset/hai/nonlinear/epistemic/Trace_Cov_J_mn_32.pdf}
%     \caption{$\mathrm{Tr}\bigl(\Sigma_{\hat{J}_{32}^t}\bigr)$}\label{fig:traceJ32}
%   \end{subfigure}

%   \caption{Nonlinear Exper. on HAI: Trace of the covariance for the off-diagonal blocks of the Jacobian matrix $J$  for different $\Sigma_{W}^t$}
%   \label{fig:trace_cov_offdiag_J_hai_epistemic}
% \end{figure}



%%%%%%%%%%%%%%%%%%%%%%%%%%SWaT%%%%%%%%%%%%%%%%%%%%%%%%%%%%%%%%%%%%%%%%%%%%%%%%%%%%%%
% \begin{figure}[H]
%   \centering
%   % Row 1 (i = 1, j = 2,3,4,5)
%   \begin{subfigure}[b]{0.25\columnwidth}
%     \centering
%     \includegraphics[width=\textwidth]{Appendix/Figures/RealworldDataset/swat/aleatoric/Trace_Cov_A_mn_12.pdf}
%     \caption{$\mathrm{Tr}(\Sigma_{\hat{A}_{12}^t})$}
%   \end{subfigure}%
%   \begin{subfigure}[b]{0.25\columnwidth}
%     \centering
%     \includegraphics[width=\textwidth]{Appendix/Figures/RealworldDataset/swat/aleatoric/Trace_Cov_A_mn_13.pdf}
%     \caption{$\mathrm{Tr}(\Sigma_{\hat{A}_{13}^t})$}
%   \end{subfigure}%
%   \begin{subfigure}[b]{0.25\columnwidth}
%     \centering
%     \includegraphics[width=\textwidth]{Appendix/Figures/RealworldDataset/swat/aleatoric/Trace_Cov_A_mn_14.pdf}
%     \caption{$\mathrm{Tr}(\Sigma_{\hat{A}_{14}^t})$}
%   \end{subfigure}%
%   \begin{subfigure}[b]{0.25\columnwidth}
%     \centering
%     \includegraphics[width=\textwidth]{Appendix/Figures/RealworldDataset/swat/aleatoric/Trace_Cov_A_mn_15.pdf}
%     \caption{$\mathrm{Tr}(\Sigma_{\hat{A}_{15}^t})$}
%   \end{subfigure}

%   \vskip\baselineskip
%   % Row 2 (i = 2, j = 1,3,4,5)
%   \begin{subfigure}[b]{0.25\columnwidth}
%     \centering
%     \includegraphics[width=\textwidth]{Appendix/Figures/RealworldDataset/swat/aleatoric/Trace_Cov_A_mn_21.pdf}
%     \caption{$\mathrm{Tr}(\Sigma_{\hat{A}_{21}^t})$}
%   \end{subfigure}%
%   \begin{subfigure}[b]{0.25\columnwidth}
%     \centering
%     \includegraphics[width=\textwidth]{Appendix/Figures/RealworldDataset/swat/aleatoric/Trace_Cov_A_mn_23.pdf}
%     \caption{$\mathrm{Tr}(\Sigma_{\hat{A}_{23}^t})$}
%   \end{subfigure}%
%   \begin{subfigure}[b]{0.25\columnwidth}
%     \centering
%     \includegraphics[width=\textwidth]{Appendix/Figures/RealworldDataset/swat/aleatoric/Trace_Cov_A_mn_24.pdf}
%     \caption{$\mathrm{Tr}(\Sigma_{\hat{A}_{24}^t})$}
%   \end{subfigure}%
%   \begin{subfigure}[b]{0.25\columnwidth}
%     \centering
%     \includegraphics[width=\textwidth]{Appendix/Figures/RealworldDataset/swat/aleatoric/Trace_Cov_A_mn_25.pdf}
%     \caption{$\mathrm{Tr}(\Sigma_{\hat{A}_{25}^t})$}
%   \end{subfigure}

%   \vskip\baselineskip
%   % Row 3 (i = 3, j = 1,2,4,5)
%   \begin{subfigure}[b]{0.25\columnwidth}
%     \centering
%     \includegraphics[width=\textwidth]{Appendix/Figures/RealworldDataset/swat/aleatoric/Trace_Cov_A_mn_31.pdf}
%     \caption{$\mathrm{Tr}(\Sigma_{\hat{A}_{31}^t})$}
%   \end{subfigure}%
%   \begin{subfigure}[b]{0.25\columnwidth}
%     \centering
%     \includegraphics[width=\textwidth]{Appendix/Figures/RealworldDataset/swat/aleatoric/Trace_Cov_A_mn_32.pdf}
%     \caption{$\mathrm{Tr}(\Sigma_{\hat{A}_{32}^t})$}
%   \end{subfigure}%
%   \begin{subfigure}[b]{0.25\columnwidth}
%     \centering
%     \includegraphics[width=\textwidth]{Appendix/Figures/RealworldDataset/swat/aleatoric/Trace_Cov_A_mn_34.pdf}
%     \caption{$\mathrm{Tr}(\Sigma_{\hat{A}_{34}^t})$}
%   \end{subfigure}%
%   \begin{subfigure}[b]{0.25\columnwidth}
%     \centering
%     \includegraphics[width=\textwidth]{Appendix/Figures/RealworldDataset/swat/aleatoric/Trace_Cov_A_mn_35.pdf}
%     \caption{$\mathrm{Tr}(\Sigma_{\hat{A}_{35}^t})$}
%   \end{subfigure}

%   \vskip\baselineskip
%   % Row 4 (i = 4, j = 1,2,3,5)
%   \begin{subfigure}[b]{0.25\columnwidth}
%     \centering
%     \includegraphics[width=\textwidth]{Appendix/Figures/RealworldDataset/swat/aleatoric/Trace_Cov_A_mn_41.pdf}
%     \caption{$\mathrm{Tr}(\Sigma_{\hat{A}_{41}^t})$}
%   \end{subfigure}%
%   \begin{subfigure}[b]{0.25\columnwidth}
%     \centering
%     \includegraphics[width=\textwidth]{Appendix/Figures/RealworldDataset/swat/aleatoric/Trace_Cov_A_mn_42.pdf}
%     \caption{$\mathrm{Tr}(\Sigma_{\hat{A}_{42}^t})$}
%   \end{subfigure}%
%   \begin{subfigure}[b]{0.25\columnwidth}
%     \centering
%     \includegraphics[width=\textwidth]{Appendix/Figures/RealworldDataset/swat/aleatoric/Trace_Cov_A_mn_43.pdf}
%     \caption{$\mathrm{Tr}(\Sigma_{\hat{A}_{43}^t})$}
%   \end{subfigure}%
%   \begin{subfigure}[b]{0.25\columnwidth}
%     \centering
%     \includegraphics[width=\textwidth]{Appendix/Figures/RealworldDataset/swat/aleatoric/Trace_Cov_A_mn_45.pdf}
%     \caption{$\mathrm{Tr}(\Sigma_{\hat{A}_{45}^t})$}
%   \end{subfigure}

%   \vskip\baselineskip
%   % Row 5 (i = 5, j = 1,2,3,4)
%   \begin{subfigure}[b]{0.25\columnwidth}
%     \centering
%     \includegraphics[width=\textwidth]{Appendix/Figures/RealworldDataset/swat/aleatoric/Trace_Cov_A_mn_51.pdf}
%     \caption{$\mathrm{Tr}(\Sigma_{\hat{A}_{51}^t})$}
%   \end{subfigure}%
%   \begin{subfigure}[b]{0.25\columnwidth}
%     \centering
%     \includegraphics[width=\textwidth]{Appendix/Figures/RealworldDataset/swat/aleatoric/Trace_Cov_A_mn_52.pdf}
%     \caption{$\mathrm{Tr}(\Sigma_{\hat{A}_{52}^t})$}
%   \end{subfigure}%
%   \begin{subfigure}[b]{0.25\columnwidth}
%     \centering
%     \includegraphics[width=\textwidth]{Appendix/Figures/RealworldDataset/swat/aleatoric/Trace_Cov_A_mn_53.pdf}
%     \caption{$\mathrm{Tr}(\Sigma_{\hat{A}_{53}^t})$}
%   \end{subfigure}%
%   \begin{subfigure}[b]{0.25\columnwidth}
%     \centering
%     \includegraphics[width=\textwidth]{Appendix/Figures/RealworldDataset/swat/aleatoric/Trace_Cov_A_mn_54.pdf}
%     \caption{$\mathrm{Tr}(\Sigma_{\hat{A}_{54}^t})$}
%   \end{subfigure}

%   \caption{Trace of the covariance for each off-diagonal block of the $A$ matrix for different regimes of $\Sigma_{y_m}^t$ on SWaT dataset}
%   \label{fig:trace_cov_offdiag_A_swat}
% \end{figure}

% \begin{figure}[H]
%   \centering
%   % Row 1 (i = 1, j = 2,3,4,5)
%   \begin{subfigure}[b]{0.25\columnwidth}
%     \centering
%     \includegraphics[width=\textwidth]{Appendix/Figures/RealworldDataset/swat/aleatoric/L2_Norm_Avg_Error_12.pdf}
%     \caption{$\|\mu_{\hat{A}_{12}^t}-A_{12}\|_2$}
%   \end{subfigure}%
%   \begin{subfigure}[b]{0.25\columnwidth}
%     \centering
%     \includegraphics[width=\textwidth]{Appendix/Figures/RealworldDataset/swat/aleatoric/L2_Norm_Avg_Error_13.pdf}
%     \caption{$\|\mu_{\hat{A}_{13}^t}-A_{13}\|_2$}
%   \end{subfigure}%
%   \begin{subfigure}[b]{0.25\columnwidth}
%     \centering
%     \includegraphics[width=\textwidth]{Appendix/Figures/RealworldDataset/swat/aleatoric/L2_Norm_Avg_Error_14.pdf}
%     \caption{$\|\mu_{\hat{A}_{14}^t}-A_{14}\|_2$}
%   \end{subfigure}%
%   \begin{subfigure}[b]{0.25\columnwidth}
%     \centering
%     \includegraphics[width=\textwidth]{Appendix/Figures/RealworldDataset/swat/aleatoric/L2_Norm_Avg_Error_15.pdf}
%     \caption{$\|\mu_{\hat{A}_{15}^t}-A_{15}\|_2$}
%   \end{subfigure}

%   \vskip\baselineskip
%   % Row 2 (i = 2, j = 1,3,4,5)
%   \begin{subfigure}[b]{0.25\columnwidth}
%     \centering
%     \includegraphics[width=\textwidth]{Appendix/Figures/RealworldDataset/swat/aleatoric/L2_Norm_Avg_Error_21.pdf}
%     \caption{$\|\mu_{\hat{A}_{21}^t}-A_{21}\|_2$}
%   \end{subfigure}%
%   \begin{subfigure}[b]{0.25\columnwidth}
%     \centering
%     \includegraphics[width=\textwidth]{Appendix/Figures/RealworldDataset/swat/aleatoric/L2_Norm_Avg_Error_23.pdf}
%     \caption{$\|\mu_{\hat{A}_{23}^t}-A_{23}\|_2$}
%   \end{subfigure}%
%   \begin{subfigure}[b]{0.25\columnwidth}
%     \centering
%     \includegraphics[width=\textwidth]{Appendix/Figures/RealworldDataset/swat/aleatoric/L2_Norm_Avg_Error_24.pdf}
%     \caption{$\|\mu_{\hat{A}_{24}^t}-A_{24}\|_2$}
%   \end{subfigure}%
%   \begin{subfigure}[b]{0.25\columnwidth}
%     \centering
%     \includegraphics[width=\textwidth]{Appendix/Figures/RealworldDataset/swat/aleatoric/L2_Norm_Avg_Error_25.pdf}
%     \caption{$\|\mu_{\hat{A}_{25}^t}-A_{25}\|_2$}
%   \end{subfigure}

%   \vskip\baselineskip
%   % Row 3 (i = 3, j = 1,2,4,5)
%   \begin{subfigure}[b]{0.25\columnwidth}
%     \centering
%     \includegraphics[width=\textwidth]{Appendix/Figures/RealworldDataset/swat/aleatoric/L2_Norm_Avg_Error_31.pdf}
%     \caption{$\|\mu_{\hat{A}_{31}^t}-A_{31}\|_2$}
%   \end{subfigure}%
%   \begin{subfigure}[b]{0.25\columnwidth}
%     \centering
%     \includegraphics[width=\textwidth]{Appendix/Figures/RealworldDataset/swat/aleatoric/L2_Norm_Avg_Error_32.pdf}
%     \caption{$\|\mu_{\hat{A}_{32}^t}-A_{32}\|_2$}
%   \end{subfigure}%
%   \begin{subfigure}[b]{0.25\columnwidth}
%     \centering
%     \includegraphics[width=\textwidth]{Appendix/Figures/RealworldDataset/swat/aleatoric/L2_Norm_Avg_Error_34.pdf}
%     \caption{$\|\mu_{\hat{A}_{34}^t}-A_{34}\|_2$}
%   \end{subfigure}%
%   \begin{subfigure}[b]{0.25\columnwidth}
%     \centering
%     \includegraphics[width=\textwidth]{Appendix/Figures/RealworldDataset/swat/aleatoric/L2_Norm_Avg_Error_35.pdf}
%     \caption{$\|\mu_{\hat{A}_{35}^t}-A_{35}\|_2$}
%   \end{subfigure}

%   \vskip\baselineskip
%   % Row 4 (i = 4, j = 1,2,3,5)
%   \begin{subfigure}[b]{0.25\columnwidth}
%     \centering
%     \includegraphics[width=\textwidth]{Appendix/Figures/RealworldDataset/swat/aleatoric/L2_Norm_Avg_Error_41.pdf}
%     \caption{$\|\mu_{\hat{A}_{41}^t}-A_{41}\|_2$}
%   \end{subfigure}%
%   \begin{subfigure}[b]{0.25\columnwidth}
%     \centering
%     \includegraphics[width=\textwidth]{Appendix/Figures/RealworldDataset/swat/aleatoric/L2_Norm_Avg_Error_42.pdf}
%     \caption{$\|\mu_{\hat{A}_{42}^t}-A_{42}\|_2$}
%   \end{subfigure}%
%   \begin{subfigure}[b]{0.25\columnwidth}
%     \centering
%     \includegraphics[width=\textwidth]{Appendix/Figures/RealworldDataset/swat/aleatoric/L2_Norm_Avg_Error_43.pdf}
%     \caption{$\|\mu_{\hat{A}_{43}^t}-A_{43}\|_2$}
%   \end{subfigure}%
%   \begin{subfigure}[b]{0.25\columnwidth}
%     \centering
%     \includegraphics[width=\textwidth]{Appendix/Figures/RealworldDataset/swat/aleatoric/L2_Norm_Avg_Error_45.pdf}
%     \caption{$\|\mu_{\hat{A}_{45}^t}-A_{45}\|_2$}
%   \end{subfigure}

%   \vskip\baselineskip
%   % Row 5 (i = 5, j = 1,2,3,4)
%   \begin{subfigure}[b]{0.25\columnwidth}
%     \centering
%     \includegraphics[width=\textwidth]{Appendix/Figures/RealworldDataset/swat/aleatoric/L2_Norm_Avg_Error_51.pdf}
%     \caption{$\|\mu_{\hat{A}_{51}^t}-A_{51}\|_2$}
%   \end{subfigure}%
%   \begin{subfigure}[b]{0.25\columnwidth}
%     \centering
%     \includegraphics[width=\textwidth]{Appendix/Figures/RealworldDataset/swat/aleatoric/L2_Norm_Avg_Error_52.pdf}
%     \caption{$\|\mu_{\hat{A}_{52}^t}-A_{52}\|_2$}
%   \end{subfigure}%
%   \begin{subfigure}[b]{0.25\columnwidth}
%     \centering
%     \includegraphics[width=\textwidth]{Appendix/Figures/RealworldDataset/swat/aleatoric/L2_Norm_Avg_Error_53.pdf}
%     \caption{$\|\mu_{\hat{A}_{53}^t}-A_{53}\|_2$}
%   \end{subfigure}%
%   \begin{subfigure}[b]{0.25\columnwidth}
%     \centering
%     \includegraphics[width=\textwidth]{Appendix/Figures/RealworldDataset/swat/aleatoric/L2_Norm_Avg_Error_54.pdf}
%     \caption{$\|\mu_{\hat{A}_{54}^t}-A_{54}\|_2$}
%   \end{subfigure}

%   \caption{Average $L_2$ norm error of each off-diagonal block of the $5\times5$ matrix $A$ for different regimes of $\Sigma_{y_m}^t$ on SWaT dataset}
%   \label{fig:L2_error_offdiag_A_swat}
% \end{figure}


% %%%%%%%%%%%%%%%%%%%SWaT Sigma_Amn %%%%%%%%%%%%%%%%%%%%%%%%%%%%%%%%%%%%%%%%%%%%
% \begin{figure}[H]
%   \centering
%   % Row 1 (i=1, j=2,3,4,5)
%   \begin{subfigure}[b]{0.25\columnwidth}
%     \centering
%     \includegraphics[width=\textwidth]{Appendix/Figures/RealworldDataset/swat/epistemic/sigma_Amn/Trace_Cov_A_mn_12.pdf}
%     \caption{$\mathrm{Tr}(\Sigma_{\hat{A}_{12}^t})$}
%   \end{subfigure}%
%   \begin{subfigure}[b]{0.25\columnwidth}
%     \centering
%     \includegraphics[width=\textwidth]{Appendix/Figures/RealworldDataset/swat/epistemic/sigma_Amn/Trace_Cov_A_mn_13.pdf}
%     \caption{$\mathrm{Tr}(\Sigma_{\hat{A}_{13}^t})$}
%   \end{subfigure}%
%   \begin{subfigure}[b]{0.25\columnwidth}
%     \centering
%     \includegraphics[width=\textwidth]{Appendix/Figures/RealworldDataset/swat/epistemic/sigma_Amn/Trace_Cov_A_mn_14.pdf}
%     \caption{$\mathrm{Tr}(\Sigma_{\hat{A}_{14}^t})$}
%   \end{subfigure}%
%   \begin{subfigure}[b]{0.25\columnwidth}
%     \centering
%     \includegraphics[width=\textwidth]{Appendix/Figures/RealworldDataset/swat/epistemic/sigma_Amn/Trace_Cov_A_mn_15.pdf}
%     \caption{$\mathrm{Tr}(\Sigma_{\hat{A}_{15}^t})$}
%   \end{subfigure}

%   \vskip\baselineskip
%   % Row 2 (i=2, j=1,3,4,5)
%   \begin{subfigure}[b]{0.25\columnwidth}
%     \centering
%     \includegraphics[width=\textwidth]{Appendix/Figures/RealworldDataset/swat/epistemic/sigma_Amn/Trace_Cov_A_mn_21.pdf}
%     \caption{$\mathrm{Tr}(\Sigma_{\hat{A}_{21}^t})$}
%   \end{subfigure}%
%   \begin{subfigure}[b]{0.25\columnwidth}
%     \centering
%     \includegraphics[width=\textwidth]{Appendix/Figures/RealworldDataset/swat/epistemic/sigma_Amn/Trace_Cov_A_mn_23.pdf}
%     \caption{$\mathrm{Tr}(\Sigma_{\hat{A}_{23}^t})$}
%   \end{subfigure}%
%   \begin{subfigure}[b]{0.25\columnwidth}
%     \centering
%     \includegraphics[width=\textwidth]{Appendix/Figures/RealworldDataset/swat/epistemic/sigma_Amn/Trace_Cov_A_mn_24.pdf}
%     \caption{$\mathrm{Tr}(\Sigma_{\hat{A}_{24}^t})$}
%   \end{subfigure}%
%   \begin{subfigure}[b]{0.25\columnwidth}
%     \centering
%     \includegraphics[width=\textwidth]{Appendix/Figures/RealworldDataset/swat/epistemic/sigma_Amn/Trace_Cov_A_mn_25.pdf}
%     \caption{$\mathrm{Tr}(\Sigma_{\hat{A}_{25}^t})$}
%   \end{subfigure}

%   \vskip\baselineskip
%   % Row 3 (i=3, j=1,2,4,5)
%   \begin{subfigure}[b]{0.25\columnwidth}
%     \centering
%     \includegraphics[width=\textwidth]{Appendix/Figures/RealworldDataset/swat/epistemic/sigma_Amn/Trace_Cov_A_mn_31.pdf}
%     \caption{$\mathrm{Tr}(\Sigma_{\hat{A}_{31}^t})$}
%   \end{subfigure}%
%   \begin{subfigure}[b]{0.25\columnwidth}
%     \centering
%     \includegraphics[width=\textwidth]{Appendix/Figures/RealworldDataset/swat/epistemic/sigma_Amn/Trace_Cov_A_mn_32.pdf}
%     \caption{$\mathrm{Tr}(\Sigma_{\hat{A}_{32}^t})$}
%   \end{subfigure}%
%   \begin{subfigure}[b]{0.25\columnwidth}
%     \centering
%     \includegraphics[width=\textwidth]{Appendix/Figures/RealworldDataset/swat/epistemic/sigma_Amn/Trace_Cov_A_mn_34.pdf}
%     \caption{$\mathrm{Tr}(\Sigma_{\hat{A}_{34}^t})$}
%   \end{subfigure}%
%   \begin{subfigure}[b]{0.25\columnwidth}
%     \centering
%     \includegraphics[width=\textwidth]{Appendix/Figures/RealworldDataset/swat/epistemic/sigma_Amn/Trace_Cov_A_mn_35.pdf}
%     \caption{$\mathrm{Tr}(\Sigma_{\hat{A}_{35}^t})$}
%   \end{subfigure}

%   \vskip\baselineskip
%   % Row 4 (i=4, j=1,2,3,5)
%   \begin{subfigure}[b]{0.25\columnwidth}
%     \centering
%     \includegraphics[width=\textwidth]{Appendix/Figures/RealworldDataset/swat/epistemic/sigma_Amn/Trace_Cov_A_mn_41.pdf}
%     \caption{$\mathrm{Tr}(\Sigma_{\hat{A}_{41}^t})$}
%   \end{subfigure}%
%   \begin{subfigure}[b]{0.25\columnwidth}
%     \centering
%     \includegraphics[width=\textwidth]{Appendix/Figures/RealworldDataset/swat/epistemic/sigma_Amn/Trace_Cov_A_mn_42.pdf}
%     \caption{$\mathrm{Tr}(\Sigma_{\hat{A}_{42}^t})$}
%   \end{subfigure}%
%   \begin{subfigure}[b]{0.25\columnwidth}
%     \centering
%     \includegraphics[width=\textwidth]{Appendix/Figures/RealworldDataset/swat/epistemic/sigma_Amn/Trace_Cov_A_mn_43.pdf}
%     \caption{$\mathrm{Tr}(\Sigma_{\hat{A}_{43}^t})$}
%   \end{subfigure}%
%   \begin{subfigure}[b]{0.25\columnwidth}
%     \centering
%     \includegraphics[width=\textwidth]{Appendix/Figures/RealworldDataset/swat/epistemic/sigma_Amn/Trace_Cov_A_mn_45.pdf}
%     \caption{$\mathrm{Tr}(\Sigma_{\hat{A}_{45}^t})$}
%   \end{subfigure}

%   \vskip\baselineskip
%   % Row 5 (i=5, j=1,2,3,4)
%   \begin{subfigure}[b]{0.25\columnwidth}
%     \centering
%     \includegraphics[width=\textwidth]{Appendix/Figures/RealworldDataset/swat/epistemic/sigma_Amn/Trace_Cov_A_mn_51.pdf}
%     \caption{$\mathrm{Tr}(\Sigma_{\hat{A}_{51}^t})$}
%   \end{subfigure}%
%   \begin{subfigure}[b]{0.25\columnwidth}
%     \centering
%     \includegraphics[width=\textwidth]{Appendix/Figures/RealworldDataset/swat/epistemic/sigma_Amn/Trace_Cov_A_mn_52.pdf}
%     \caption{$\mathrm{Tr}(\Sigma_{\hat{A}_{52}^t})$}
%   \end{subfigure}%
%   \begin{subfigure}[b]{0.25\columnwidth}
%     \centering
%     \includegraphics[width=\textwidth]{Appendix/Figures/RealworldDataset/swat/epistemic/sigma_Amn/Trace_Cov_A_mn_53.pdf}
%     \caption{$\mathrm{Tr}(\Sigma_{\hat{A}_{53}^t})$}
%   \end{subfigure}%
%   \begin{subfigure}[b]{0.25\columnwidth}
%     \centering
%     \includegraphics[width=\textwidth]{Appendix/Figures/RealworldDataset/swat/epistemic/sigma_Amn/Trace_Cov_A_mn_54.pdf}
%     \caption{$\mathrm{Tr}(\Sigma_{\hat{A}_{54}^t})$}
%   \end{subfigure}

%   \caption{Trace of the covariance for each off-diagonal block of the $A$ matrix for different regimes of $\Sigma_{\hat{A}_{mn}}^0$ on SWaT dataset}
%   \label{fig:trace_cov_offdiag_A_swat_Sigma}
% \end{figure}

% \begin{figure}[H]
%   \centering
%   % Theta covariance for 5 components
%   \begin{subfigure}[b]{0.17\columnwidth}
%     \centering
%     \includegraphics[width=\textwidth]{Appendix/Figures/RealworldDataset/swat/epistemic/sigma_Amn/Trace_Cov_theta_1.pdf}
%     \caption{$\mathrm{Tr}(\Sigma_{\theta_1}^t)$}
%   \end{subfigure}%
%   \begin{subfigure}[b]{0.17\columnwidth}
%     \centering
%     \includegraphics[width=\textwidth]{Appendix/Figures/RealworldDataset/swat/epistemic/sigma_Amn/Trace_Cov_theta_2.pdf}
%     \caption{$\mathrm{Tr}(\Sigma_{\theta_2}^t)$}
%   \end{subfigure}%
%   \begin{subfigure}[b]{0.17\columnwidth}
%     \centering
%     \includegraphics[width=\textwidth]{Appendix/Figures/RealworldDataset/swat/epistemic/sigma_Amn/Trace_Cov_theta_3.pdf}
%     \caption{$\mathrm{Tr}(\Sigma_{\theta_3}^t)$}
%   \end{subfigure}%
%   \begin{subfigure}[b]{0.17\columnwidth}
%     \centering
%     \includegraphics[width=\textwidth]{Appendix/Figures/RealworldDataset/swat/epistemic/sigma_Amn/Trace_Cov_theta_4.pdf}
%     \caption{$\mathrm{Tr}(\Sigma_{\theta_4}^t)$}
%   \end{subfigure}
%   \begin{subfigure}[b]{0.17\columnwidth}
%     \centering
%     \includegraphics[width=\textwidth]{Appendix/Figures/RealworldDataset/swat/epistemic/sigma_Amn/Trace_Cov_theta_5.pdf}
%     \caption{$\mathrm{Tr}(\Sigma_{\theta_5}^t)$}
%   \end{subfigure}%
%   % \begin{subfigure}[b]{0.25\columnwidth}\centering~\end{subfigure}%
%   % \begin{subfigure}[b]{0.25\columnwidth}\centering~\end{subfigure}%
%   % \begin{subfigure}[b]{0.25\columnwidth}\centering~\end{subfigure}

%   \caption{Trace of the covariance of the local model parameters $\theta$ for each of the five components during FedGC learning for different regimes of $\Sigma_{\hat{A}_{mn}}^0$ on SWaT dataset, plotted vs.\ iteration $t$.}
%   \label{fig:trace_cov_theta_swat}
% \end{figure}

% \begin{figure}[H]
%   \centering
%   % L2 norm error 20 off-diagonals
%   % Row 1 (1,2,3,4)
%   \begin{subfigure}[b]{0.25\columnwidth}
%     \centering
%     \includegraphics[width=\textwidth]{Appendix/Figures/RealworldDataset/swat/epistemic/sigma_Amn/L2_Norm_Avg_Error_12.pdf}
%     \caption{$\|\mu_{\hat{A}_{12}^t}-A_{12}\|_2$}
%   \end{subfigure}%
%   \begin{subfigure}[b]{0.25\columnwidth}
%     \centering
%     \includegraphics[width=\textwidth]{Appendix/Figures/RealworldDataset/swat/epistemic/sigma_Amn/L2_Norm_Avg_Error_13.pdf}
%     \caption{$\|\mu_{\hat{A}_{13}^t}-A_{13}\|_2$}
%   \end{subfigure}%
%   \begin{subfigure}[b]{0.25\columnwidth}
%     \centering
%     \includegraphics[width=\textwidth]{Appendix/Figures/RealworldDataset/swat/epistemic/sigma_Amn/L2_Norm_Avg_Error_14.pdf}
%     \caption{$\|\mu_{\hat{A}_{14}^t}-A_{14}\|_2$}
%   \end{subfigure}%
%   \begin{subfigure}[b]{0.25\columnwidth}
%     \centering
%     \includegraphics[width=\textwidth]{Appendix/Figures/RealworldDataset/swat/epistemic/sigma_Amn/L2_Norm_Avg_Error_15.pdf}
%     \caption{$\|\mu_{\hat{A}_{15}^t}-A_{15}\|_2$}
%   \end{subfigure}

%   \vskip\baselineskip
%   % Row 2 (2,1,3,4,5)
%   \begin{subfigure}[b]{0.25\columnwidth}
%     \centering
%     \includegraphics[width=\textwidth]{Appendix/Figures/RealworldDataset/swat/epistemic/sigma_Amn/L2_Norm_Avg_Error_21.pdf}
%     \caption{$\|\mu_{\hat{A}_{21}^t}-A_{21}\|_2$}
%   \end{subfigure}%
%   \begin{subfigure}[b]{0.25\columnwidth}
%     \centering
%     \includegraphics[width=\textwidth]{Appendix/Figures/RealworldDataset/swat/epistemic/sigma_Amn/L2_Norm_Avg_Error_23.pdf}
%     \caption{$\|\mu_{\hat{A}_{23}^t}-A_{23}\|_2$}
%   \end{subfigure}%
%   \begin{subfigure}[b]{0.25\columnwidth}
%     \centering
%     \includegraphics[width=\textwidth]{Appendix/Figures/RealworldDataset/swat/epistemic/sigma_Amn/L2_Norm_Avg_Error_24.pdf}
%     \caption{$\|\mu_{\hat{A}_{24}^t}-A_{24}\|_2$}
%   \end{subfigure}%
%   \begin{subfigure}[b]{0.25\columnwidth}
%     \centering
%     \includegraphics[width=\textwidth]{Appendix/Figures/RealworldDataset/swat/epistemic/sigma_Amn/L2_Norm_Avg_Error_25.pdf}
%     \caption{$\|\mu_{\hat{A}_{25}^t}-A_{25}\|_2$}
%   \end{subfigure}

%   \vskip\baselineskip
%   % Row 3 (3,1,2,4,5)
%   \begin{subfigure}[b]{0.25\columnwidth}
%     \centering
%     \includegraphics[width=\textwidth]{Appendix/Figures/RealworldDataset/swat/epistemic/sigma_Amn/L2_Norm_Avg_Error_31.pdf}
%     \caption{$\|\mu_{\hat{A}_{31}^t}-A_{31}\|_2$}
%   \end{subfigure}%
%   \begin{subfigure}[b]{0.25\columnwidth}
%     \centering
%     \includegraphics[width=\textwidth]{Appendix/Figures/RealworldDataset/swat/epistemic/sigma_Amn/L2_Norm_Avg_Error_32.pdf}
%     \caption{$\|\mu_{\hat{A}_{32}^t}-A_{32}\|_2$}
%   \end{subfigure}%
%   \begin{subfigure}[b]{0.25\columnwidth}
%     \centering
%     \includegraphics[width=\textwidth]{Appendix/Figures/RealworldDataset/swat/epistemic/sigma_Amn/L2_Norm_Avg_Error_34.pdf}
%     \caption{$\|\mu_{\hat{A}_{34}^t}-A_{34}\|_2$}
%   \end{subfigure}%
%   \begin{subfigure}[b]{0.25\columnwidth}
%     \centering
%     \includegraphics[width=\textwidth]{Appendix/Figures/RealworldDataset/swat/epistemic/sigma_Amn/L2_Norm_Avg_Error_35.pdf}
%     \caption{$\|\mu_{\hat{A}_{35}^t}-A_{35}\|_2$}
%   \end{subfigure}

%   \vskip\baselineskip
%   % Row 4 (4,1,2,3,5)
%   \begin{subfigure}[b]{0.25\columnwidth}
%     \centering
%     \includegraphics[width=\textwidth]{Appendix/Figures/RealworldDataset/swat/epistemic/sigma_Amn/L2_Norm_Avg_Error_41.pdf}
%     \caption{$\|\mu_{\hat{A}_{41}^t}-A_{41}\|_2$}
%   \end{subfigure}%
%   \begin{subfigure}[b]{0.25\columnwidth}
%     \centering
%     \includegraphics[width=\textwidth]{Appendix/Figures/RealworldDataset/swat/epistemic/sigma_Amn/L2_Norm_Avg_Error_42.pdf}
%     \caption{$\|\mu_{\hat{A}_{42}^t}-A_{42}\|_2$}
%   \end{subfigure}%
%   \begin{subfigure}[b]{0.25\columnwidth}
%     \centering
%     \includegraphics[width=\textwidth]{Appendix/Figures/RealworldDataset/swat/epistemic/sigma_Amn/L2_Norm_Avg_Error_43.pdf}
%     \caption{$\|\mu_{\hat{A}_{43}^t}-A_{43}\|_2$}
%   \end{subfigure}%
%   \begin{subfigure}[b]{0.25\columnwidth}
%     \centering
%     \includegraphics[width=\textwidth]{Appendix/Figures/RealworldDataset/swat/epistemic/sigma_Amn/L2_Norm_Avg_Error_45.pdf}
%     \caption{$\|\mu_{\hat{A}_{45}^t}-A_{45}\|_2$}
%   \end{subfigure}

%   \vskip\baselineskip
%   % Row 5 (5,1,2,3,4)
%   \begin{subfigure}[b]{0.25\columnwidth}
%     \centering
%     \includegraphics[width=\textwidth]{Appendix/Figures/RealworldDataset/swat/epistemic/sigma_Amn/L2_Norm_Avg_Error_51.pdf}
%     \caption{$\|\mu_{\hat{A}_{51}^t}-A_{51}\|_2$}
%   \end{subfigure}%
%   \begin{subfigure}[b]{0.25\columnwidth}
%     \centering
%     \includegraphics[width=\textwidth]{Appendix/Figures/RealworldDataset/swat/epistemic/sigma_Amn/L2_Norm_Avg_Error_52.pdf}
%     \caption{$\|\mu_{\hat{A}_{52}^t}-A_{52}\|_2$}
%   \end{subfigure}%
%   \begin{subfigure}[b]{0.25\columnwidth}
%     \centering
%     \includegraphics[width=\textwidth]{Appendix/Figures/RealworldDataset/swat/epistemic/sigma_Amn/L2_Norm_Avg_Error_53.pdf}
%     \caption{$\|\mu_{\hat{A}_{53}^t}-A_{53}\|_2$}
%   \end{subfigure}%
%   \begin{subfigure}[b]{0.25\columnwidth}
%     \centering
%     \includegraphics[width=\textwidth]{Appendix/Figures/RealworldDataset/swat/epistemic/sigma_Amn/L2_Norm_Avg_Error_54.pdf}
%     \caption{$\|\mu_{\hat{A}_{54}^t}-A_{54}\|_2$}
%   \end{subfigure}

%   \caption{Average $L_2$ norm error of each off-diagonal block of the $A$ matrix for different regimes of $\Sigma_{\hat{A}_{mn}}^0$ on SWaT dataset}
%   \label{fig:L2_error_offdiag_A_swat_Sigma}
% \end{figure}




% %%%%%%%%%%%%%%%%%%%%%%% SWaT sigma_theta %%%%%%%%%%%%%%%%%%%%%%%%%%%%%%%%%

% % — Figure: A off‐diagonal covariance (5×5 → 20 off‐diagonals, 4 per row) —
% \begin{figure}[H]
%   \centering
%   % Row 1 (i=1, j=2,3,4,5)
%   \begin{subfigure}[b]{0.25\columnwidth}
%     \centering
%     \includegraphics[width=\textwidth]{Appendix/Figures/RealworldDataset/swat/epistemic/sigma_theta/Trace_Cov_A_mn_12.pdf}
%     \caption{$\mathrm{Tr}(\Sigma_{\hat{A}_{12}^t})$}
%   \end{subfigure}%
%   \begin{subfigure}[b]{0.25\columnwidth}
%     \centering
%     \includegraphics[width=\textwidth]{Appendix/Figures/RealworldDataset/swat/epistemic/sigma_theta/Trace_Cov_A_mn_13.pdf}
%     \caption{$\mathrm{Tr}(\Sigma_{\hat{A}_{13}^t})$}
%   \end{subfigure}%
%   \begin{subfigure}[b]{0.25\columnwidth}
%     \centering
%     \includegraphics[width=\textwidth]{Appendix/Figures/RealworldDataset/swat/epistemic/sigma_theta/Trace_Cov_A_mn_14.pdf}
%     \caption{$\mathrm{Tr}(\Sigma_{\hat{A}_{14}^t})$}
%   \end{subfigure}%
%   \begin{subfigure}[b]{0.25\columnwidth}
%     \centering
%     \includegraphics[width=\textwidth]{Appendix/Figures/RealworldDataset/swat/epistemic/sigma_theta/Trace_Cov_A_mn_15.pdf}
%     \caption{$\mathrm{Tr}(\Sigma_{\hat{A}_{15}^t})$}
%   \end{subfigure}
  
%   \vskip\baselineskip
%   % Row 2 (i=2, j=1,3,4,5)
%   \begin{subfigure}[b]{0.25\columnwidth}
%     \centering
%     \includegraphics[width=\textwidth]{Appendix/Figures/RealworldDataset/swat/epistemic/sigma_theta/Trace_Cov_A_mn_21.pdf}
%     \caption{$\mathrm{Tr}(\Sigma_{\hat{A}_{21}^t})$}
%   \end{subfigure}%
%   \begin{subfigure}[b]{0.25\columnwidth}
%     \centering
%     \includegraphics[width=\textwidth]{Appendix/Figures/RealworldDataset/swat/epistemic/sigma_theta/Trace_Cov_A_mn_23.pdf}
%     \caption{$\mathrm{Tr}(\Sigma_{\hat{A}_{23}^t})$}
%   \end{subfigure}%
%   \begin{subfigure}[b]{0.25\columnwidth}
%     \centering
%     \includegraphics[width=\textwidth]{Appendix/Figures/RealworldDataset/swat/epistemic/sigma_theta/Trace_Cov_A_mn_24.pdf}
%     \caption{$\mathrm{Tr}(\Sigma_{\hat{A}_{24}^t})$}
%   \end{subfigure}%
%   \begin{subfigure}[b]{0.25\columnwidth}
%     \centering
%     \includegraphics[width=\textwidth]{Appendix/Figures/RealworldDataset/swat/epistemic/sigma_theta/Trace_Cov_A_mn_25.pdf}
%     \caption{$\mathrm{Tr}(\Sigma_{\hat{A}_{25}^t})$}
%   \end{subfigure}

%   \vskip\baselineskip
%   % Row 3 (i=3, j=1,2,4,5)
%   \begin{subfigure}[b]{0.25\columnwidth}
%     \centering
%     \includegraphics[width=\textwidth]{Appendix/Figures/RealworldDataset/swat/epistemic/sigma_theta/Trace_Cov_A_mn_31.pdf}
%     \caption{$\mathrm{Tr}(\Sigma_{\hat{A}_{31}^t})$}
%   \end{subfigure}%
%   \begin{subfigure}[b]{0.25\columnwidth}
%     \centering
%     \includegraphics[width=\textwidth]{Appendix/Figures/RealworldDataset/swat/epistemic/sigma_theta/Trace_Cov_A_mn_32.pdf}
%     \caption{$\mathrm{Tr}(\Sigma_{\hat{A}_{32}^t})$}
%   \end{subfigure}%
%   \begin{subfigure}[b]{0.25\columnwidth}
%     \centering
%     \includegraphics[width=\textwidth]{Appendix/Figures/RealworldDataset/swat/epistemic/sigma_theta/Trace_Cov_A_mn_34.pdf}
%     \caption{$\mathrm{Tr}(\Sigma_{\hat{A}_{34}^t})$}
%   \end{subfigure}%
%   \begin{subfigure}[b]{0.25\columnwidth}
%     \centering
%     \includegraphics[width=\textwidth]{Appendix/Figures/RealworldDataset/swat/epistemic/sigma_theta/Trace_Cov_A_mn_35.pdf}
%     \caption{$\mathrm{Tr}(\Sigma_{\hat{A}_{35}^t})$}
%   \end{subfigure}

%   \vskip\baselineskip
%   % Row 4 (i=4, j=1,2,3,5)
%   \begin{subfigure}[b]{0.25\columnwidth}
%     \centering
%     \includegraphics[width=\textwidth]{Appendix/Figures/RealworldDataset/swat/epistemic/sigma_theta/Trace_Cov_A_mn_41.pdf}
%     \caption{$\mathrm{Tr}(\Sigma_{\hat{A}_{41}^t})$}
%   \end{subfigure}%
%   \begin{subfigure}[b]{0.25\columnwidth}
%     \centering
%     \includegraphics[width=\textwidth]{Appendix/Figures/RealworldDataset/swat/epistemic/sigma_theta/Trace_Cov_A_mn_42.pdf}
%     \caption{$\mathrm{Tr}(\Sigma_{\hat{A}_{42}^t})$}
%   \end{subfigure}%
%   \begin{subfigure}[b]{0.25\columnwidth}
%     \centering
%     \includegraphics[width=\textwidth]{Appendix/Figures/RealworldDataset/swat/epistemic/sigma_theta/Trace_Cov_A_mn_43.pdf}
%     \caption{$\mathrm{Tr}(\Sigma_{\hat{A}_{43}^t})$}
%   \end{subfigure}%
%   \begin{subfigure}[b]{0.25\columnwidth}
%     \centering
%     \includegraphics[width=\textwidth]{Appendix/Figures/RealworldDataset/swat/epistemic/sigma_theta/Trace_Cov_A_mn_45.pdf}
%     \caption{$\mathrm{Tr}(\Sigma_{\hat{A}_{45}^t})$}
%   \end{subfigure}

%   \vskip\baselineskip
%   % Row 5 (i=5, j=1,2,3,4)
%   \begin{subfigure}[b]{0.25\columnwidth}
%     \centering
%     \includegraphics[width=\textwidth]{Appendix/Figures/RealworldDataset/swat/epistemic/sigma_theta/Trace_Cov_A_mn_51.pdf}
%     \caption{$\mathrm{Tr}(\Sigma_{\hat{A}_{51}^t})$}
%   \end{subfigure}%
%   \begin{subfigure}[b]{0.25\columnwidth}
%     \centering
%     \includegraphics[width=\textwidth]{Appendix/Figures/RealworldDataset/swat/epistemic/sigma_theta/Trace_Cov_A_mn_52.pdf}
%     \caption{$\mathrm{Tr}(\Sigma_{\hat{A}_{52}^t})$}
%   \end{subfigure}%
%   \begin{subfigure}[b]{0.25\columnwidth}
%     \centering
%     \includegraphics[width=\textwidth]{Appendix/Figures/RealworldDataset/swat/epistemic/sigma_theta/Trace_Cov_A_mn_53.pdf}
%     \caption{$\mathrm{Tr}(\Sigma_{\hat{A}_{53}^t})$}
%   \end{subfigure}%
%   \begin{subfigure}[b]{0.25\columnwidth}
%     \centering
%     \includegraphics[width=\textwidth]{Appendix/Figures/RealworldDataset/swat/epistemic/sigma_theta/Trace_Cov_A_mn_54.pdf}
%     \caption{$\mathrm{Tr}(\Sigma_{\hat{A}_{54}^t})$}
%   \end{subfigure}

%   \caption{Trace of the covariance for each off-diagonal block of the $A$ matrix during FedGC learning for different regimes of $\Sigma_{\theta_m}^0$ on SWaT dataset, plotted vs.\ iteration $t$.}
%   \label{fig:trace_cov_offdiag_A_swat}
% \end{figure}

% \begin{figure}[H]
%   \centering
%   % Theta covariance for 5 components
%   \begin{subfigure}[b]{0.33\columnwidth}
%     \centering
%     \includegraphics[width=\textwidth]{Appendix/Figures/RealworldDataset/swat/epistemic/sigma_Amn/Trace_Cov_theta_1.pdf}
%     \caption{$\mathrm{Tr}(\Sigma_{\theta_1}^t)$}
%   \end{subfigure}%
%   \begin{subfigure}[b]{0.33\columnwidth}
%     \centering
%     \includegraphics[width=\textwidth]{Appendix/Figures/RealworldDataset/swat/epistemic/sigma_Amn/Trace_Cov_theta_2.pdf}
%     \caption{$\mathrm{Tr}(\Sigma_{\theta_2}^t)$}
%   \end{subfigure}%
%   \begin{subfigure}[b]{0.33\columnwidth}
%     \centering
%     \includegraphics[width=\textwidth]{Appendix/Figures/RealworldDataset/swat/epistemic/sigma_Amn/Trace_Cov_theta_3.pdf}
%     \caption{$\mathrm{Tr}(\Sigma_{\theta_3}^t)$}
%   \end{subfigure}%
%   \\
%   \begin{subfigure}[b]{0.33\columnwidth}
%     \centering
%     \includegraphics[width=\textwidth]{Appendix/Figures/RealworldDataset/swat/epistemic/sigma_Amn/Trace_Cov_theta_4.pdf}
%     \caption{$\mathrm{Tr}(\Sigma_{\theta_4}^t)$}
%   \end{subfigure}
%   \begin{subfigure}[b]{0.33\columnwidth}
%     \centering
%     \includegraphics[width=\textwidth]{Appendix/Figures/RealworldDataset/swat/epistemic/sigma_Amn/Trace_Cov_theta_5.pdf}
%     \caption{$\mathrm{Tr}(\Sigma_{\theta_5}^t)$}
%   \end{subfigure}%
%   % \begin{subfigure}[b]{0.25\columnwidth}\centering~\end{subfigure}%
%   % \begin{subfigure}[b]{0.25\columnwidth}\centering~\end{subfigure}%
%   % \begin{subfigure}[b]{0.25\columnwidth}\centering~\end{subfigure}

%   \caption{Trace of the covariance of the local model parameters $\theta$ for each of the five components during FedGC learning for different regimes of $\Sigma_{\hat{A}_{mn}}^0$ on SWaT dataset, plotted vs.\ iteration $t$.}
%   \label{fig:trace_cov_theta_swat}
% \end{figure}

% % — Figure: Theta covariance (5 components) —
% \begin{figure}[H]
%   \centering
%   % Row 1 (m=1…4)
%   \begin{subfigure}[b]{0.33\textwidth}
%     \centering
%     \includegraphics[width=\textwidth]{Appendix/Figures/RealworldDataset/swat/epistemic/sigma_theta/Trace_Cov_theta_1.pdf}
%     \caption{$\mathrm{Tr}(\Sigma_{\theta_1}^t)$}
%   \end{subfigure}%
%   \begin{subfigure}[b]{0.33\textwidth}
%     \centering
%     \includegraphics[width=\textwidth]{Appendix/Figures/RealworldDataset/swat/epistemic/sigma_theta/Trace_Cov_theta_2.pdf}
%     \caption{$\mathrm{Tr}(\Sigma_{\theta_2}^t)$}
%   \end{subfigure}%
%   \begin{subfigure}[b]{0.33\textwidth}
%     \centering
%     \includegraphics[width=\textwidth]{Appendix/Figures/RealworldDataset/swat/epistemic/sigma_theta/Trace_Cov_theta_3.pdf}
%     \caption{$\mathrm{Tr}(\Sigma_{\theta_3}^t)$}
%   \end{subfigure}%
%   \\
%   \begin{subfigure}[b]{0.33\textwidth}
%     \centering
%     \includegraphics[width=\textwidth]{Appendix/Figures/RealworldDataset/swat/epistemic/sigma_theta/Trace_Cov_theta_4.pdf}
%     \caption{$\mathrm{Tr}(\Sigma_{\theta_4}^t)$}
%   \end{subfigure}
%   % Row 2 (m=5 + blanks)
%   \begin{subfigure}[b]{0.33\textwidth}
%     \centering
%     \includegraphics[width=\textwidth]{Appendix/Figures/RealworldDataset/swat/epistemic/sigma_theta/Trace_Cov_theta_5.pdf}
%     \caption{$\mathrm{Tr}(\Sigma_{\theta_5}^t)$}
%   \end{subfigure}%
%   % \begin{subfigure}[b]{0.25\columnwidth}\centering~\end{subfigure}%
%   % \begin{subfigure}[b]{0.25\columnwidth}\centering~\end{subfigure}%
%   % \begin{subfigure}[b]{0.25\columnwidth}\centering~\end{subfigure}

%   \caption{Trace of the covariance of the local model parameters $\theta$ for each of the five components during FedGC learning for different regimes of $\Sigma_{\theta_m}^0$ on SWaT dataset, plotted vs.\ iteration $t$.}
%   \label{fig:trace_cov_theta_swat}
% \end{figure}


% % — Figure: L2 norm error (20 off-diagonals) —
% \begin{figure}[H]
%   \centering
%   % Row 1 (1→2,3,4,5)
%   \begin{subfigure}[b]{0.25\columnwidth}
%     \centering
%     \includegraphics[width=\textwidth]{Appendix/Figures/RealworldDataset/swat/epistemic/sigma_theta/L2_Norm_Avg_Error_12.pdf}
%     \caption{$\|\mu_{\hat{A}_{12}^t}-A_{12}\|_2$}
%   \end{subfigure}%
%   \begin{subfigure}[b]{0.25\columnwidth}
%     \centering
%     \includegraphics[width=\textwidth]{Appendix/Figures/RealworldDataset/swat/epistemic/sigma_theta/L2_Norm_Avg_Error_13.pdf}
%     \caption{$\|\mu_{\hat{A}_{13}^t}-A_{13}\|_2$}
%   \end{subfigure}%
%   \begin{subfigure}[b]{0.25\columnwidth}
%     \centering
%     \includegraphics[width=\textwidth]{Appendix/Figures/RealworldDataset/swat/epistemic/sigma_theta/L2_Norm_Avg_Error_14.pdf}
%     \caption{$\|\mu_{\hat{A}_{14}^t}-A_{14}\|_2$}
%   \end{subfigure}%
%   \begin{subfigure}[b]{0.25\columnwidth}
%     \centering
%     \includegraphics[width=\textwidth]{Appendix/Figures/RealworldDataset/swat/epistemic/sigma_theta/L2_Norm_Avg_Error_15.pdf}
%     \caption{$\|\mu_{\hat{A}_{15}^t}-A_{15}\|_2$}
%   \end{subfigure}

%   \vskip\baselineskip
%   % Row 2 (2→1,3,4,5)
%   \begin{subfigure}[b]{0.25\columnwidth}
%     \centering
%     \includegraphics[width=\textwidth]{Appendix/Figures/RealworldDataset/swat/epistemic/sigma_theta/L2_Norm_Avg_Error_21.pdf}
%     \caption{$\|\mu_{\hat{A}_{21}^t}-A_{21}\|_2$}
%   \end{subfigure}%
%   \begin{subfigure}[b]{0.25\columnwidth}
%     \centering
%     \includegraphics[width=\textwidth]{Appendix/Figures/RealworldDataset/swat/epistemic/sigma_theta/L2_Norm_Avg_Error_23.pdf}
%     \caption{$\|\mu_{\hat{A}_{23}^t}-A_{23}\|_2$}
%   \end{subfigure}%
%   \begin{subfigure}[b]{0.25\columnwidth}
%     \centering
%     \includegraphics[width=\textwidth]{Appendix/Figures/RealworldDataset/swat/epistemic/sigma_theta/L2_Norm_Avg_Error_24.pdf}
%     \caption{$\|\mu_{\hat{A}_{24}^t}-A_{24}\|_2$}
%   \end{subfigure}%
%   \begin{subfigure}[b]{0.25\columnwidth}
%     \centering
%     \includegraphics[width=\textwidth]{Appendix/Figures/RealworldDataset/swat/epistemic/sigma_theta/L2_Norm_Avg_Error_25.pdf}
%     \caption{$\|\mu_{\hat{A}_{25}^t}-A_{25}\|_2$}
%   \end{subfigure}

%   \vskip\baselineskip
%   % Row 3 (3→1,2,4,5)
%   \begin{subfigure}[b]{0.25\columnwidth}
%     \centering
%     \includegraphics[width=\textwidth]{Appendix/Figures/RealworldDataset/swat/epistemic/sigma_theta/L2_Norm_Avg_Error_31.pdf}
%     \caption{$\|\mu_{\hat{A}_{31}^t}-A_{31}\|_2$}
%   \end{subfigure}%
%   \begin{subfigure}[b]{0.25\columnwidth}
%     \centering
%     \includegraphics[width=\textwidth]{Appendix/Figures/RealworldDataset/swat/epistemic/sigma_theta/L2_Norm_Avg_Error_32.pdf}
%     \caption{$\|\mu_{\hat{A}_{32}^t}-A_{32}\|_2$}
%   \end{subfigure}%
%   \begin{subfigure}[b]{0.25\columnwidth}
%     \centering
%     \includegraphics[width=\textwidth]{Appendix/Figures/RealworldDataset/swat/epistemic/sigma_theta/L2_Norm_Avg_Error_34.pdf}
%     \caption{$\|\mu_{\hat{A}_{34}^t}-A_{34}\|_2$}
%   \end{subfigure}%
%   \begin{subfigure}[b]{0.25\columnwidth}
%     \centering
%     \includegraphics[width=\textwidth]{Appendix/Figures/RealworldDataset/swat/epistemic/sigma_theta/L2_Norm_Avg_Error_35.pdf}
%     \caption{$\|\mu_{\hat{A}_{35}^t}-A_{35}\|_2$}
%   \end{subfigure}

%   \vskip\baselineskip
%   % Row 4 (4→1,2,3,5)
%   \begin{subfigure}[b]{0.25\columnwidth}
%     \centering
%     \includegraphics[width=\textwidth]{Appendix/Figures/RealworldDataset/swat/epistemic/sigma_theta/L2_Norm_Avg_Error_41.pdf}
%     \caption{$\|\mu_{\hat{A}_{41}^t}-A_{41}\|_2$}
%   \end{subfigure}%
%   \begin{subfigure}[b]{0.25\columnwidth}
%     \centering
%     \includegraphics[width=\textwidth]{Appendix/Figures/RealworldDataset/swat/epistemic/sigma_theta/L2_Norm_Avg_Error_42.pdf}
%     \caption{$\|\mu_{\hat{A}_{42}^t}-A_{42}\|_2$}
%   \end{subfigure}%
%   \begin{subfigure}[b]{0.25\columnwidth}
%     \centering
%     \includegraphics[width=\textwidth]{Appendix/Figures/RealworldDataset/swat/epistemic/sigma_theta/L2_Norm_Avg_Error_43.pdf}
%     \caption{$\|\mu_{\hat{A}_{43}^t}-A_{43}\|_2$}
%   \end{subfigure}%
%   \begin{subfigure}[b]{0.25\columnwidth}
%     \centering
%     \includegraphics[width=\textwidth]{Appendix/Figures/RealworldDataset/swat/epistemic/sigma_theta/L2_Norm_Avg_Error_45.pdf}
%     \caption{$\|\mu_{\hat{A}_{45}^t}-A_{45}\|_2$}
%   \end{subfigure}

%   \vskip\baselineskip
%   % Row 5 (5→1,2,3,4)
%   \begin{subfigure}[b]{0.25\columnwidth}
%     \centering
%     \includegraphics[width=\textwidth]{Appendix/Figures/RealworldDataset/swat/epistemic/sigma_theta/L2_Norm_Avg_Error_51.pdf}
%     \caption{$\|\mu_{\hat{A}_{51}^t}-A_{51}\|_2$}
%   \end{subfigure}%
%   \begin{subfigure}[b]{0.25\columnwidth}
%     \centering
%     \includegraphics[width=\textwidth]{Appendix/Figures/RealworldDataset/swat/epistemic/sigma_theta/L2_Norm_Avg_Error_52.pdf}
%     \caption{$\|\mu_{\hat{A}_{52}^t}-A_{52}\|_2$}
%   \end{subfigure}%
%   \begin{subfigure}[b]{0.25\columnwidth}
%     \centering
%     \includegraphics[width=\textwidth]{Appendix/Figures/RealworldDataset/swat/epistemic/sigma_theta/L2_Norm_Avg_Error_53.pdf}
%     \caption{$\|\mu_{\hat{A}_{53}^t}-A_{53}\|_2$}
%   \end{subfigure}%
%   \begin{subfigure}[b]{0.25\columnwidth}
%     \centering
%     \includegraphics[width=\textwidth]{Appendix/Figures/RealworldDataset/swat/epistemic/sigma_theta/L2_Norm_Avg_Error_54.pdf}
%     \caption{$\|\mu_{\hat{A}_{54}^t}-A_{54}\|_2$}
%   \end{subfigure}

%   \caption{Average $L_2$ norm error of each off-diagonal block of the $A$ matrix during FedGC learning for different regimes of $\Sigma_{\theta_m}^0$ on SWaT dataset, plotted vs.\ iteration $t$.}
%   \label{fig:L2_error_offdiag_A_swat}
% \end{figure}
