# Supplementary material for: Uncertainty Quantification in Federated Granger Causality Learning
Source: arXiv:2602.13004 source file (2026-10-08)
Supplement: Supplementary file 3 [file assumptions.tex]

% \textbf{(A1) \textit{Stochasticity}.}
% For every client \(m\), the {\textit{client model parameter}} $\theta_m^t$, and {\textit{client data}} $y_m^t$ are random variables. The local client state \(
% \hat h_{m,c}^{\,t}\;\;\text{is deterministic}
% \). Consequently, the only randomness entering the augmented states
% \(\hat h_{m,a}^{\,t}=\hat h_{m,c}^{\,t}+\theta_m^{\,t}y_m^{\,t}\)
% comes from  \(\theta_m^{\,t}\) and \(y_m^{\,t}\).
% In the server model, the Granger causal estimation $\hat{A}_{mn}^t$ $\forall n \neq m$ (also called the {\textit{server model parameter}}) is random. 

% \textbf{(A2) \textit{Model Parameters}.}\;
% The server parameters $A_{mn}^{\,t}$, $n\neq m$, are mutually independent across block-rows and times. 
% As a consequence, for any distinct clients $m \neq n$, the induced parameters $\theta_m^t$ and $\theta_n^t$ have zero cross-covariance at every time $t$, i.e. $\operatorname{Cov}(\theta_m^t,\theta_n^t) = 0, \hspace{0.2cm} \forall m\neq n,\; \forall t.$ We formally establish this result in Lemma~\ref{lemma:client_grad_cov_means}, and Proposition~\ref{prop:theta_indep}.

% \textbf{(A3) \textit{Prior}.}
% The initial server and client parameters are independent, i.e., 
% \(
% \hat{A}_{mn}^{\,0}\;\perp\!\!\!\perp\;
% \theta_m^{\,0}
% \), and the initial client parameters are uncorrelated, i.e., 
% \(
% \operatorname{Cov}(\theta_m^{\,0},\,\theta_n^{\,0})=0  \hspace{0.2cm} \forall n \neq m.
% \)

% \textbf{(A4) \textit{Stationarity}.}
% Client data are weakly stationary with time-invariant first and second moments:
% $\operatorname{E}[y_m^{\,t}]=\mu_{y_m},$
% $\operatorname{Var}(y_m^{\,t})=\Sigma_{y_m},
% \forall t$
% \begin{itemize}
%     \item Assumption \textbf{(A4)} is required only for the training data used in uncertainty propagation analysis and steady-state characterization. The testing data used in downstream evaluation need not satisfy weak stationarity.
    
%     \item We additionally discuss relaxations of Assumption \textbf{(A4)} in Appendix~\ref{appendix:relaxing_stationary}.
% \end{itemize}
